# Supplementary material for: Neural Rough Differential Equations for Long Time Series
Source: arXiv:2009.08295 source file (2021-06-21)
Supplement: Supplementary file 1 [file other.tex]

% \newpage

% %This stuff will appear in the NSDEs paper

% %\section{Derivation of the adjoint controlled differential equation}
% %
% %\begin{theorem}
% %Consider the controlled differential equation,
% %\begin{equation}
% %dy_t = \sum_{i=1}^d f_i(y_t, \theta)\,dX_t^{(i)},
% %\label{eq:cde_for_adjoint}
% %\end{equation}
% %where $X:[0,T]\rightarrow\R^d$ has finite length and each $f_i : \R^n \times \R^m \rightarrow \R^n$ is bounded and differentiable with bounded first derivatives. Let $L$ denote a differentiable loss function.
% %Then the adjoint process
% %\begin{equation}
% %a(t) = \frac{dL(y_T)}{dy_t}\,,
% %\label{eq:adjoint_process_def}
% %\end{equation}
% %satisfies the following backwards CDE
% %\begin{equation}
% %da(t) = -\sum_{i=1}^d \nabla f_i(y_t, \theta)a(t)\,d\overleftarrow{X}_t^{(i)},
% %\label{eq:adjoint_process_cde}
% %\end{equation}
% %where $\overleftarrow{X}$ is the time-reversed control path. That is, $\overleftarrow{X}_t := X_{T-t}\,$ for $t\in[0,T]$.
% %\end{theorem}
% %\begin{proof}
% %Since the path $\overleftarrow{X}$ has finite length, the flow map $\Psi_{s,t} : \R^n\rightarrow \R^n$ for the time-reversed CDE on $[s,t]$ is well-defined.
% %\begin{equation}
% %\Psi_{s,t}(y) = y - \int_s^t \Psi_{u,t}(y)\,d\overleftarrow{X}_u.
% %\label{eq:backwards_cde}
% %\end{equation}
% %
% %It was shown by Theorem 4.4. in \cite{friz2010multidimensional} that CDE flows have directional derivatives. As a result of this theorem, taking the gradient of (\ref{eq:backwards_cde}) is possible and gives
% %\begin{equation}
% %\nabla\Psi_{s,t}(y) = I_d -  \int_s^t \,dM_u^{t, y}\big(\nabla\Psi_{u,t}(y)\big),
% %\label{eq:almost_adjoint_cde}
% %\end{equation}
% %where for $u\in[s,t]$, the process $M^{t, y}$ is given by
% %\begin{equation}
% %M_u^{t, y} =  \sum_{i=1}^d\int_u^t \nabla f_i(\Psi_{v,t}(y), \theta)\,d\overleftarrow{X}_v^{(i)}.\nonumber
% %\end{equation}
% %For the rest of the proof, we will slightly abuse notation and write integrals with respect to $M^{t, y}$ as
% %\begin{equation}
% %\int_s^t \big(\cdots\big) \,dM_u^{t, y},\nonumber
% %\end{equation}
% %Since we view $M^{t,y}$ as a finite dimensional path, we believe this integral notation should be helpful.
% %We shall use the notation $\|\gamma\|_{1-var;[s,t]}$ to denote the length (or $1$-variation) of a path $\gamma : [s,t] \rightarrow \R^k$,
% %\begin{equation}
% %\|\gamma\|_{1\text{-var;}[s,t]} := \sup_{\mathcal{D}}\sum_{i} \|\gamma_{t_{i+1}} - \gamma_{t_i}\|,\nonumber
% %\end{equation}
% %where $\|\cdot\|$ is a norm on $\R^k$ and the supremum is taken over all partitions $\mathcal{D}$ of $[s,t]$.
% %
% %It is worth noting that since $u\mapsto \nabla f_i(y_u, \theta)$ is continuous, it is bounded for $u\in[s,t]$. As a result, $M^{u, y_u}$ has finite length on $[s,u]$ and there exists a constant $C_1 > 0$ (depending only on $t$) such that
% %\begin{equation}
% %\|M^{u, y_u}\|_{1-var;[s,u]}\leq C_1 \|X\|_{1-var;[s,t]},
% %\label{eq:1var_est}
% %\end{equation}
% %for $u\in[s,t]$ with $s$ and $t$ sufficiently close together.
% %
% %Applying the chain rule to the adjoint process $a(t) = \frac{dL(y_T)}{dy_t} $ gives
% %\begin{equation}
% %a(t) = \frac{dL}{dy_t} = \frac{dy_s}{dy_t}\frac{dL}{dy_s} = \nabla\Psi_{s,t}(y_t)a(s).
% %\label{eq:adjoint_chain}
% %\end{equation}
% %
% %Note that the existence of the derivative $\frac{dy_T}{dy_t}$ follows from Theorem 2.17 in \cite{li2006smoothness}.
% %
% %Thus, substituting (\ref{eq:almost_adjoint_cde}) into the above gives,
% %\begin{align}
% %a(t) & = \nabla\Psi_{s,t}(y_t)a(s)\nonumber\\
% %& = a(s) -  \bigg(\int_s^t \nabla\Psi_{u,t}(y_t)\,dM_u^{t, y_t}\bigg)a(s),
% %\label{eq:almost_adjoint_cde2}
% %\end{align}
% %
% %We can rewrite (\ref{eq:almost_adjoint_cde}) as the following linear CDE:
% %\begin{align*}
% %dz_u & = - z_u\,d\overleftarrow{M}_u^{v, y_v},\\
% %z_0 & = I_d.
% %\end{align*}
% %where $z_u := \nabla \Psi_{v - u,v}(y_v)$ for $s\leq u\leq v$.
% %
% %Since $\overleftarrow{M}^{v, y_v}$ has finite length, it follows by Davie's lemma for linear CDEs (Lemma 10.56 in \cite{friz2010multidimensional}), that there exists a constant $C_2 > 0$ such that
% %\begin{equation}
% %\|\nabla \Psi_{u,v}(y_v) - I_d\m\| \leq C_2 \|M^{v, y_v}\|_{1-var;[s,v]}.\nonumber
% %\end{equation}
% %for $s<u<v<t$ whenever $s$ is sufficiently close to $t$.
% %
% %Hence by the $1$-variation estimate (\ref{eq:1var_est}), there exists a constant $C_3 > 0$ depending only on $t$, such that
% %\begin{equation}
% %\|\nabla\Psi_{u,v}(y_v) - I_d\m\| \leq C_3\|X\|_{1-var;[s,t]},
% %\label{eq:davie_lemma}
% %\end{equation}
% %for $s<u<v<t$ whenever $s$ is sufficiently close to $t$.
% %
% %Since $a$ is continuous, it is bounded on $[s,t]$ and so it follows from (\ref{eq:adjoint_chain}) with the estimate (\ref{eq:davie_lemma}) that
% %\begin{align}
% %\|a(u) - a(v)\| & = \| \nabla\Psi_{v,u}(y_u)a(v) - a(v)\| \nonumber\\[3pt]
% %& \leq \|a(v)\|\|\nabla\Psi_{v,u}(y_u) - I_d\m\| \nonumber\\[3pt]
% %& \leq C_4\|X\|_{1-var;[s,t]},\label{eq:easy_length_estimate}
% %\end{align}
% %and
% %\begin{align}
% %\bigg\|\int_u^t a(v) - \nabla\Psi_{v,t}(y_t)a(v)\,dM_v^{t, y_t}\bigg\| & \leq \sup_{v\in[s,t]}\Big(\|a(v)\|\,\|\nabla\Psi_{v,t}(y_t) - I_d\m\|\Big)\|M^{t, y_t}\|_{1-var;[s,t]}\nonumber\\
% %& \leq C_5\|X\|_{1-var;[s,t]}^2,\label{eq:square_length_estimate}
% %\end{align}
% %for $s\leq u\leq v\leq t$ where the constants $C_4$ and $C_5$ only depends on $t$ (provided that $\epsilon := t- s$ is sufficiently small). Using equation (\ref{eq:almost_adjoint_cde2}) for the adjoint process along with the above estimates gives
% %\begin{align*}
% %&\bigg\|a(t) - \bigg(a(s) -  \int_s^t a(u)\,dM_u^{t, y_t}\bigg)\bigg\|\\
% %&\mm = \bigg\|\int_s^t \Big(a(u) - \nabla\Psi_{u,t}(y_t)a(s)\Big)\,dM_u^{t, y_t}\bigg\|\\
% %&\mm \leq \bigg\|\int_s^t \Big(a(u) - \nabla\Psi_{u,t}(y_t)a(u)\Big)\,dM_u^{t, y_t}\bigg\| + \bigg\|\int_s^t \Big(\nabla\Psi_{u,t}(y_t)(a(u)-a(s))\Big)\,dM_u^{t, y_t}\bigg\|\\
% %&\mm \leq C_5\|X\|_{1-var;[s,t]}^2 + \bigg(C_1\,C_4\sup_{u\in[s,t]}\|\nabla\Psi_{u,t}(y_t)\|\bigg)\|X\|_{1-var;[s,t]}^2.
% %\end{align*}
% %In other words, for a fixed $t$, we have
% %\begin{equation}
% %a(t) = a(s) -  \int_s^t a(u)\,dM_u^{t, y_t} + O\Big(\|X\|_{1-var;[s,t]}^2\Big),
% %\label{eq:square_length_remainder}
% %\end{equation}
% %provided that $s$ is sufficiently close to $t$. Letting $s\rightarrow t^-$ and applying the chain rule to $M^{t, y_t}$ gives
% %\begin{align*}
% %da(t) = -\sum_{i=1}^d \nabla f_i(y_t, \theta)a(t)\,d\overleftarrow{X}_t^{(i)},
% %\end{align*}
% %as required.
% %\end{proof}

% %\newpage

% \section{A universal approximation theorem for (linear) CDEs and log-ODEs}
% \label{appendix:universal}

% In this section, we shall prove that the linear controlled differential equations and their log-ODE approximations are sufficiently rich to uniformly approximate functions on (compact) path spaces.
% The key idea is that we should augment the state space of  the response $Y$ to include latent variables. 

% \medbreak
% \begin{theorem}[A universal approximation theorem for linear log-ODEs]\label{thm:approxthm}
% Let $\mathcal{X}$ be a compact set of continuous finite variation paths $X:[0,T]\rightarrow \R^d$. We say that paths $X$ and $Y$ are equivalent if at least one of the following holds:
% \begin{enumerate}
% \item $X - Y$ is a constant path.
% \item $X$ can be reparametrized to give $Y$. That is, there exists a strictly increasing function $\varphi : [0,T]\rightarrow [0,T]$ such that $X_{\varphi(t)} = Y_t$.
% \item Removing ``tree-like'' excursions from $X$ and $Y$ gives two equivalent (under 1 and  2) paths $\widetilde{X}$ and $\widetilde{Y}$. Tree-like paths have trivial integrals and their precise definition is given in \cite{hambly2010sigunique}.
% \end{enumerate}

% We will assume that no two paths in $\mathcal{X}$ are equivalent. In addition, we consider the followings spaces:
% \begin{itemize}
% \item Let $C(\mathcal{X}, \R)$ denote the algebra of real-valued continuous functions on $\mathcal{X}$ equipped with the topology of uniform convergence.

% \item Let $C^{lin}(\mathcal{X}, \R)$ denote the space of functions $p$ on $\mathcal{X}$ with the form $p(X) = P(Sig_{0,T}^{N}(X))$, where $P : T^N(\R^d) \rightarrow \R\m$ is a linear functional on a truncated tensor algebra.

% \item Let $C^{cde}(\mathcal{X}, \R)$ be the space of ``projected linear CDE solutions''. That is, any function that maps a path $X\in\mathcal{X}$ to the projection onto $\R$ of the solution to a linear CDE driven by $X$.

% \item Let $C^{log}(\mathcal{X}, \R)$ denote the space of ``projected linear log-ODE approximations'' That is, any function which can be expressed as the projection onto $\R$ of the ODE solution $z(1)$ where $z^\prime = F(z)\big(LogSig_{0,T}^{N}(X)\big)$ with $z(0) = z_0\in\R^n$ and $F : \R^n\rightarrow L\big(T^N(\R^d),\R^n\big)\m$.

% \item Let $C^{Lie}(\mathcal{X}, \R)$ be the subset of $C^{log}(\mathcal{X}, \R)$ where the function $F : \R^n\rightarrow L\big(T^N(\R^d),\R^n\big)\m$ takes the form (\ref{eq:linearlogode}), and so is defined from vector fields $\{f_1,\cdots, f_d\}$ where $f_i : \R^n\rightarrow\R^n$.
% \end{itemize}

% Then $C^{lin}(\mathcal{X}, \R)$, $C^{Lie}(\mathcal{X}, \R)$, $C^{log}(\mathcal{X}, \R)$ and $C^{cde}(\mathcal{X}, \R)$ are all dense subsets of $C(\mathcal{X}, \R)$.
% \end{theorem}

% \begin{proof}
% To begin, we will consider the following map
% \begin{equation}
% \varphi: X \mapsto Sig_{0,T}(X),
% \label{eq:sig_map}
% \end{equation}
% for paths $X\in\mathcal{X}$. Since each the paths in $\mathcal{X}$ have finite variation, the (extended) signature $Sig_{0,T}(X)$ can be defined via Riemann-Stieltjes integration. Moreover, it follows from the main results of \cite{hambly2010sigunique} (Theorem 4 and its corollaries) that any two finite variation paths $X$ and $Y$ are equivalent if and only if they have the same signature. Therefore $\varphi$ is a well defined bijection from $\mathcal{X}$ onto $\varphi(\mathcal{X})$.

% Note that $\mathcal{X}$ is endowed with the $1$-variation norm
% \begin{equation}
% \|X\|_{1\text{-Var;}[0,T]} := \sup_{\mathcal{D}}\sum_{k} \|X_{t_{k+1}} - X_{t_{k}}\|,
% \label{eq:one_var_norm}
% \end{equation}
% where $\|\cdot\|$ is a norm on $\R^d$ and the supremum is taken over all partitions $\mathcal{D}$ of $[0,T]$. It is also worth noting that the iterated integrals in $Sig_{0,T}(X)$ experience a factorial decay by Proposition 2.2. in \cite{roughpath2007notes} (further asymptotic estimates are given in \cite{horatio2020sig}),
% \begin{equation}
% \bigg\|\int_0^t\int_0^{t_{n-1}}\cdots \int_0^{t_{2}} X_{t_1}^{(i_1)}\,dX_{t_2}^{(i_2)} \cdots dX_{t_n}^{(i_n)}\bigg\|\leq \frac{1}{n!}\|X\|_{1\text{-Var;}[0,T]}^n\,,
% \label{eq:fact_decay}
% \end{equation}

% for each multi index $I = (i_1,\cdots, i_n)\in \{1,\cdots,d\}^d$.

% Therefore, $\varphi(\mathcal{X})$ can be endowed with the projective norm:
% \begin{equation}
% \big\|Sig_{0,T}(X)\big\|_1 := \sum_{n\geq 1}\,\sum_{I = (i_1,\cdots, i_n)\in \{1,\cdots,d\}^n} \big\|S_{0,T}^{(I)}\big\|,
% \label{eq:proj_norm}
% \end{equation}

% By the standard properties of Riemann-Stieltjes integration and the factorial decay (\ref{eq:fact_decay}), we see that $\varphi$ is a continuous bijection from $\mathcal{X}$ to $\varphi(\mathcal{X})$. Since $\mathcal{X}$ is a compact metric space, $\varphi$ is a homeomorphism.

% So for any function $f\in C(\mathcal{X}, \R)$, there exists a unique continuous function $g := f \circ \varphi^{-1}$ such that
% \begin{equation}
% f(X) = g(Sig_{0,T}(X)).
% \label{eq:function_equiv}
% \end{equation}

% Thus, it suffices to show that the space of linear functionals $F : \varphi(\mathcal{X}) \rightarrow \R$ are dense in $C(\varphi(\mathcal{X}), \R)$.

% By Lemma 9.4 in \cite{lyons2014streams},
% the space of linear functionals on the ``signature space'' $\varphi(\mathcal{X})$ will form an algebra (under pointwise multiplication) that contains the constant functions and separates points.
% The proof of this result uses the fact that finite variation paths satisfy an integration by parts formula
% which then corresponds to a certain shuffle algebra on noncommutative polynomials with $d$ variables.

% Hence by the Stone-Weierstrass theorem, the space of linear functionals on $\varphi(\mathcal{X})$ are dense in $C(\varphi(\mathcal{X}), \R)$. Moreover, by (\ref{eq:function_equiv}), we see that any function $f\in C(\mathcal{X}, \R)$ is equivalent to a function $g\in C(\varphi(\mathcal{X}), \R)$. Therefore, it is a direct consequence that $C^{lin}(\mathcal{X}, \R)$ is dense in $C(\mathcal{X}, \R)$.
% The result follows since $C^{lin}(\mathcal{X}, \R) \subseteq C^{Lie}(\mathcal{X}, \R) \subseteq C^{log}(\mathcal{X}, \R) \subseteq C^{cde}(\mathcal{X}, \R)$ by Theorem \ref{thm:set_inclusions}.
% \end{proof}

% To complete the above proof, we require Theorem \ref{thm:linear_cde}, where we show that any linear functional of the path signature $Sig_{0,T}(X)$ can be represented as both the solution of a CDE and its log-ODE approximation.
% The key idea is that we augment the state space of the response $Y$ to include latent variables,
% which will encode the ``derivatives'' of the response $Y$ with respect to the driving path $X$.

% \begin{theorem}\label{thm:set_inclusions} We have the following set inclusions:
% \begin{equation}
% C^{lin}(\mathcal{X}, \R) \subsetneq C^{Lie}(\mathcal{X}, \R) \subseteq C^{log}(\mathcal{X}, \R) \subseteq C^{cde}(\mathcal{X}, \R).
% \label{eq:set_inclusions}
% \end{equation}
% \end{theorem}
% \begin{proof}
% Note that $C^{Lie}(\mathcal{X}, \R) \subseteq C^{log}(\mathcal{X}, \R)$ follows directly from their definitions in Theorem \ref{thm:approxthm}. We shall prove (\ref{eq:set_inclusions}) using lemmas (\ref{thm:linear_cde}) and (\ref{thm:ode_subset_cde}) given below:

% \begin{lemma}
% \label{thm:linear_cde}
% Suppose that $X : [0,T] \rightarrow \R^d$ is a finite variation path and let $F : T^N(\R^d) \rightarrow \R$ be a linear functional on the truncated tensor algebra $T^N(\R^d)$. Then $Y_t = F(S_{0,t}^{N}(X))$ can be augmented to the solution $\widetilde{Y} = (Y, Z)$ of a linear controlled differential equation,
% \begin{equation}
% d\widetilde{Y}_t = \widetilde{F}(Y_t)\,dX_t,
% \label{eq:linear_functional_cde}
% \end{equation}
% where $\widetilde{Y}$ takes values in $\R^n$ and $\widetilde{F} : \R^n\rightarrow L(\R^d, \R^n)$ is linear. In addition, the controlled differential equation (\ref{eq:linear_functional_cde}) can be constructed so that the solution $\widetilde{Y}_t$ coincides with the solution at $u=1$ of the following log-ODE:
% \begin{align}
% \frac{dy}{du} & = \sum_{k=1}^N\widetilde{F}^k(y_u)\,\pi_k\Big(\log^N\big(S_{0,t}^N(X)\big)\Big),\label{eq:linearlogode}\\
% y_0 & = \widetilde{Y}_0,\nonumber
% \end{align}
% where $\pi_k : T^N(\R^d)\rightarrow (\R^d)^{\otimes k}$ is the projection map onto $\big(\R^d\big)^{\otimes k}$, $\log^N$ is the logarithm map on
% $\{a\in T^N(\R^d) : \pi_0(a) > 0\}$ and the linear map $\widetilde{F}^k : \R^n\rightarrow L\big((\R^d)^{\otimes k}, \R^n\big)$ is defined recursively:
% \begin{align*}
% \widetilde{F}^{1}(y)(x) & :=  \widetilde{F}(y)x,\\
% \widetilde{F}^{(k+1)}(y)(x_1\otimes \cdots \otimes x_{k+1}) & :=  \widetilde{F}(y)\big(\widetilde{F}^k(y)(x_1\otimes \cdots \otimes x_k)\big)x_{k+1},
% \end{align*}
% for $y\in\R^n$ and $x_1, \cdots, x_{k+1}\in\R^d$.
% \end{lemma}
% \begin{proof}
% We proceed by induction on $N$. For $N = 1$, we can express $Y$ as
% \begin{equation}
% Y_t = Y_0 + a_1 X_t^{(1)} + \cdots + a_d X_t^{(d)},\nonumber
% \end{equation}
% where $a_1, \cdots, a_d\in\R$. We set $Z = 1$, so that $\widetilde{Y} = (Y, Z)$ solves
% \begin{equation}
% d\begin{pmatrix} Y_t\\ Z_t\end{pmatrix}
% =
% \begin{pmatrix} a_1 Z_t & \cdots & a_d Z_t\\[3pt] 0 & \cdots & 0 \end{pmatrix} d \begin{pmatrix} X_t^{(1)}\\ \vdots \\X_t^{(d)}\end{pmatrix},\label{eq:basecasecde}
% \end{equation}
% with the initial value
% \begin{equation}
% \widetilde{Y}_0 = \begin{pmatrix} Y_0\\ 1\end{pmatrix}.\nonumber
% \end{equation}

% We note that the matrix governing (\ref{eq:basecasecde}) is strictly upper triangular when viewed in the block form:
% \begin{equation}
% \begin{pmatrix} a_1 z & \cdots & a_d z\\[3pt] 0 & \cdots & 0 \end{pmatrix} = \begin{pmatrix} \underline{a}z\\ \underline{0}\end{pmatrix}.\label{eq:base_upper_triag}
% \end{equation}

% In any case, the log-ODE approximation (\ref{eq:linearlogode}) for the controlled differential equation (\ref{eq:basecasecde}) becomes
% \begin{equation}
% \frac{d}{du}\begin{pmatrix} y_u\\ z_u\end{pmatrix}
% =
% \begin{pmatrix} a_1 z_u & \cdots & a_d z_u\\[3pt] 0 & \cdots & 0 \end{pmatrix} \begin{pmatrix} X_t^{(1)}\\ \vdots \\X_t^{(d)}\end{pmatrix},\hspace{2.5mm} \begin{pmatrix} y_0\\ z_0\end{pmatrix} = \begin{pmatrix} Y_0\\ 1\end{pmatrix},
% \end{equation}
% which clearly coincides with $\widetilde{Y}_t$ at $u = 1$.

% Now suppose that for some $K\geq 1$, the statement of the theorem is true for $N \leq K - 1$.
% In addition, we assume the vector field for the linear CDE (\ref{eq:linear_functional_cde}) can be constructed to be strictly upper triangular
% when expressed in block matrix form with blocks of size $1\times d$. By (\ref{eq:base_upper_triag}), this will be true for $K=1$.

% We proceed by induction on $N$. For $N = K$, we can express $Y$ as
% \begin{equation}
% Y_t = \sum_{\substack{I = (i_1, \cdots, i_k)\in\{1,\cdots, d\}^k \\ 0 \leq k \leq K + 1}}F^{(i_1, \cdots, i_k)}\int_0^t\int_0^{t_{k-1}}\cdots \int_0^{t_{2}} X_{t_1}^{(i_1)}\,dX_{t_2}^{(i_2)} \cdots dX_{t_k}^{(i_k)},
% \label{eq:inductionstep1}
% \end{equation}
% where $F^I\in\R$ for a multi-index $I = (i_1, \cdots, i_k)\in\{1,\cdots d\}^k$. The process (\ref{eq:inductionstep1}) can be written as
% \begin{equation}
% Y_t = Y_0 + \sum_{j\in\{1,\cdots,d\}}\int_0^t \big(Y_s^\prime\big)^{(j)} dX_s^{(j)}.
% \label{eq:keystep1}
% \end{equation}
% where $Y^\prime$ is the $d$-dimensional process given by
% \begin{equation}
% \big(Y_t^\prime\big)^{(j)} := \sum_{\substack{I = (i_1, \cdots, i_k)\in\{1,\cdots, d\}^k \\ 0 \leq k \leq K}}F^{(i_1, \cdots, i_k,\, j)}\int_0^t\int_0^{t_{k-1}}\cdots \int_0^{t_{2}} X_{t_1}^{(i_1)}\,dX_{t_2}^{(i_2)} \cdots dX_{t_k}^{(i_k)}.
% \label{eq:keystep2}
% \end{equation}
% Note that each coordinate of $Y^\prime$ is defined by some linear functional on the truncated tensor algebra $T^{K}(\R^d)$. So by applying the induction hypothesis to each coordinate, $Y^\prime$ can be augmented to give a process $\widetilde{Y}^\prime = (Y^\prime, Z^\prime)$ that satisfies a linear controlled differential equation:
% \begin{equation}
% d\widetilde{Y}_t^\prime = \widetilde{f}\big(\widetilde{Y}_t^\prime\big)\,dX_t,\nonumber
% \end{equation}
% Therefore, we define $Z := \widetilde{Y}^\prime$ so that $\widetilde{Y} := (Y, Z)$ satisfies
% \begin{align}
% d\begin{pmatrix} Y_t\\ Z_t\end{pmatrix}
% & =
% \begin{pmatrix} \begin{pmatrix} Z_t^{(1)} &\cdots & Z_t^{(d)}\end{pmatrix} &  0 \\[3pt] 0 & \widetilde{f}(Z_t) \end{pmatrix} d \begin{pmatrix} X_t^{(1)}\\ \vdots \\X_t^{(d)}\end{pmatrix},
% \label{eq:inductionstep2}\\
% \widetilde{Y}_0 & = \begin{pmatrix} Y_0\\ \widetilde{Y}_0^\prime\end{pmatrix}.\nonumber
% \end{align}
% where we use block matrix notation in (\ref{eq:inductionstep2}). Let $\widetilde{F}$ be the linear vector field governing the CDE (\ref{eq:inductionstep2}):
% \begin{equation}
% \widetilde{F}(x) :=
% \begin{pmatrix} \begin{pmatrix} Z_t^{(1)} &\cdots & Z_t^{(d)}\end{pmatrix} &  0 \\[3pt] 0 & \widetilde{f}(Z_t) \end{pmatrix} x.\nonumber
% \end{equation}
% It is clear from our construction that $\widetilde{F}$ is strictly upper triangular when viewed as a block matrix (with blocks of size $1\times d$). As $\widetilde{F}$ is the ``$K$-th matrix'' in our induction, it is $(K+1)$-step nilpotent, i.e. $\widetilde{F}^m = 0$ for all $m\geq K + 1$. We now consider the log-ODE:
% \begin{align}
% \frac{dy}{du} & = \sum_{m=1}^K\widetilde{F}^m(y_u)\,\pi_m\Big(\log^K\big(S_{0,t}^K(X)\big)\Big),\label{eq:anotherlogode}\\
% y_0 & = \begin{pmatrix} Y_0\\ \widetilde{Y}_0^\prime\end{pmatrix}.\nonumber
% \end{align}
% Since (\ref{eq:anotherlogode}) is a linear ODE, its solution can be expressed as the exponential of the governing matrix. Due to the nilpotency of $\widetilde{F}$, we can make the following rearrangements:
% \begin{align*}
% y_1 & = \exp\left(\sum_{m=1}^K\widetilde{F}^m(\cdot)\,\pi_m\Big(\log^K\big(S_{0,t}^K(X)\big)\Big)\right) y_0\\
% & = \sum_{k=0}^\infty\frac{1}{k!}\left(\,\sum_{m=1}^\infty\widetilde{F}^m(\cdot)\,\pi_m\Big(\log\big(S_{0,t}(X)\big)\Big)\right)^k y_0\\
% & = \sum_{m=1}^\infty \widetilde{F}^m(\cdot)\,\pi_m\left(\,\sum_{k=0}^\infty\frac{1}{k!}\Big(\log\big(S_{0,t}(X)\big)\Big)^{\otimes k}\right) y_0\\
% & = \sum_{m=1}^\infty \widetilde{F}^m(\cdot)\,\pi_m\Big(\exp\Big(\log\big(S_{0,t}(X)\big)\Big)\Big) y_0\\
% & = \sum_{m=1}^K \widetilde{F}^m(y_0)\,\pi_m\big(S_{0,t}^K(X)\big).
% \end{align*}

% Hence $y_1$ is expressible as a linear functional on the truncated signature of $X$. Moreover, it is clear from our construction ((\ref{eq:keystep1}) and (\ref{eq:keystep2})) that each $\widetilde{F}^K(y_0)$ contains the coefficients of $F$ at level $k$ (provided that $\widetilde{F}^m(y_0)$ contain the correct coefficients for $1\leq m\leq K - 1$).
% \end{proof}
% \begin{lemma}
% \label{thm:ode_subset_cde}
% Let $X : [0,T] \rightarrow \R^d$ be a finite variation path and, for each $t\geq 0$, consider the ODE:
% \begin{align}
% \frac{dz^t}{du} & = F\big(LogSig_{0,t}^{N}(X)\big) z^t,\label{eq:general_linear_logode}\\[3pt]
% z^t(0) & = Y_0,\nonumber
% \end{align}
% where $Y_0\in\R^n$ and $F : T^N(\R^d) \rightarrow L\big(\R^n,\R^n\big)$ is linear. Thus $F\big(LogSig_{0,t}^{N}(X)\big)$ is an $n\times n$ matrix. Then the process $Y_t := z^t(1)$ can be augmented to the solution $\widetilde{Y} = (Y, Z)$ of a linear CDE,
% \begin{equation}
% d\widetilde{Y}_t = \widetilde{F}(Y_t)\,dX_t,
% \label{eq:linear_functional_cde2}
% \end{equation}
% where $\widetilde{Y}$ takes values in $\R^{\tilde{n}}$ for some $\tilde{n} \geq n$ and $\widetilde{F} : \R^{\tilde{n}}\rightarrow L(\R^d, \R^{\tilde{n}})$ is linear.
% \end{lemma}
% \begin{proof}
% Since the ODE (\ref{eq:general_linear_logode}) is linear, we can express its solution using the matrix exponential as
% \begin{align*}
% z^t(1) = \exp\big(F\big(LogSig_{0,t}^{N}(X)\big)\big)z^t(0),
% \end{align*}
% which is equivalent to
% \begin{align*}
% Y_t = \exp\big(F\big(LogSig_{0,t}^{N}(X)\big)\big)Y_0.
% \end{align*}

% By the shuffle product, we have that each coordinate of $LogSig_{0,t}^{N}(X)$ can be expressed as a linear combination of coordinate integrals from $Sig_{0,t}^{N}(X)$. It then immediately follows that the process $M_t := F\big(LogSig_{0,t}^{N}(X)\big)$ is simple a linear functional of the truncated signature $Sig_{0,t}^{N}(X)$. Moreover, it is always the case that $M_0 = 0$ as $LogSig_{0,0}(X) = 0$. Thus, we can express $M$ as
% \begin{equation}
% M_t = \sum_{\substack{I = (i_1, \cdots, i_k)\in\{1,\cdots, d\}^k \\ 1 \leq k \leq N}}M^{(i_1, \cdots, i_k)}\int_0^t\int_0^{t_{k-1}}\cdots \int_0^{t_{2}} X_{t_1}^{(i_1)}\,dX_{t_2}^{(i_2)} \cdots dX_{t_k}^{(i_k)},
% \label{eq:m_def}
% \end{equation}
% where each coefficient $M^{(I)}\in L(\R^n, \R^n)$ is an $n\times n$ matrix. In particular, this means that
% \begin{equation}
% M_t = \sum_{j=1}^d \int_0^t \big(M_s^\prime\big)^{(j)} dX_s^{(j)}.\label{eq:m_with_derivative}
% \end{equation}
% where the process $M^\prime : [0,T] \rightarrow L\big(\R^d, L\big(\R^n, \R^n\big)\big)$ is given by
% \begin{equation}
% \big(M_s^\prime\big)^{(j)} := \sum_{\substack{I = (i_1, \cdots, i_k, j)\in\{1,\cdots, d\}^k \\ 0 \leq k \leq N-1}}M^{(i_1, \cdots, i_k, j)}\int_0^t\int_0^{t_k}\cdots \int_0^{t_{2}} X_{t_1}^{(i_1)}\,dX_{t_2}^{(i_2)} \cdots dX_{t_k}^{(i_k)}.\nonumber
% \end{equation}

% Recall that the log-ODE process $Y_t$ can be expressed as
% \begin{equation}
% Y_t = \exp(M_t)Y_0.
% \label{eq:y_in_terms_of_m}
% \end{equation}

% It then follows from the series definition of $\exp(M_t)$ and standard properties of matrix integration
% \begin{align}
% \exp(M_t) & = \big(I_n + M_t + \frac{1}{2}M_t^2 + \cdots )\nonumber\\
% & = I_n + \bigg(M_t + \frac{1}{2}M_t^2 + \frac{1}{6}M_t^3 + \cdots \bigg)\nonumber\\
% & = I_n + \int_0^t \Big(I_n + M_s + \frac{1}{2}M_s^2 + \cdots \Big) \,dM_s\nonumber\\
% & = I_n+ \int_0^t \exp(M_s) \,dM_s\m.\label{eq:y_integral_form}
% \end{align}

% Letting $E_t = \exp(M_t)$, we see from the integral equation (\ref{eq:y_integral_form}) that
% \begin{align}
% dY_t & = \big(dZ_t\big) Y_0, \label{eq:yem_system1}\\
% dE_t & = E_t\,dM_t,\label{eq:yem_system2}\\
% dM_t & = M_t^\prime\,dX_t,\label{eq:yem_system3}
% \end{align}
% where $Z_0 = I_n$ and $M_0 = 0$.

% Since $M_t^\prime$ can be expressed as a linear functional on $Sig_{0,t}^{N}(X)$, it can be augmented to satisfy a linear CDE by Lemma \ref{thm:linear_cde}. Therefore, the system (\ref{eq:yem_system1} - \ref{eq:yem_system3}) can be expressed as a CDE driven by $X$.
% \end{proof}

% Thus, we have shown that $C^{lin}(\mathcal{X}, \R) \subseteq C^{Lie}(\mathcal{X}, \R) \subseteq C^{log}(\mathcal{X}, \R) \subseteq C^{cde}(\mathcal{X}, \R)$ and so all that remains is to show that the first set inclusion is actually strict.

% Suppose $X^{(i)}$ is non-constant for all $i\in\{1,\cdots,d\}$. We can define a process $Y^{(i)}:[0,T]\rightarrow\R^d$ by
% \begin{equation}
% Y_t^{(i)} := Y_0^{(i)}\exp\big(X_t^{(i)}\big),
% \end{equation}
% where $Y_0^{(i)}\in\R$ is assumed to be non-zero. Then $Y_t^{(i)} = z_1$ where $z$ satisfies the log-ODE:
% \begin{align*}
% \frac{dz}{du} & = \big(X_t^{(i)}\big)z,\\
% z_0 & = Y_0^{(i)}.
% \end{align*}
% Since $Y^{(i)}$ is not a polynomial function of $X_t^{(i)}$, it immediately follows that it cannot be expressed using a finite linear functional on $Sig_{0,t}\big(X^{(i)}\big) = \big(1, X_t, \frac{1}{2}\big(X_t^{(i)}\big)^2, \cdots, \frac{1}{N!}\big(X_t^{(i)}\big)^N, \cdots\big)$. Hence,
% the multidimensional process $Y = (Y^{(1)}, \cdots, Y^{(d)})$ can be represented by the solution of a log-ODE but not by a linear functional on $Sig_{0,t}^N(X)$. Therefore $C^{lin}(\mathcal{X}, \R) \neq C^{Lie}(\mathcal{X}, \R)$ as required.
% \end{proof}

% % I dont' think this section is actually relevant.

% %\section{Convergence of the log-ODE method for rough differential equations}
% %
% %In this section, we shall present ``rough path'' error estimates for the log-ODE method. In addition, we will discuss the case when the vector fields governing the rough differential equation are linear.\medbreak
% %
% %\begin{theorem}[Lemma 15 in \cite{logode2014estimate}]\label{thm:logODEthm}
% %Consider the rough differential equation on $[0,T]$:
% %\begin{align}
% %dY_t & = f(Y_t)\,dX_t,\label{eq:RDE}\\
% %Y_0 & = \xi,\nonumber
% %\end{align}
% %where we make the following assumptions:
% %\begin{itemize}
% %\item $X$ is a geometric $p$-rough path in $\R^d$, that is $X : [0,T] \rightarrow T^{\floor{p}}(\R^d)$ is a continuous path in the tensor algebra
% %$T^{\floor{p}}(\R^d) := \R \oplus \R^d \oplus \big(\R^d\big)^{\otimes 2} \oplus \cdots \oplus \big(\R^d\big)^{\otimes \floor{p}}$ with increments
% %\begin{align}
% %X_{s,t} & = \Big(1, X_{s,t}^1, X_{s,t}^2, \cdots, X_{s,t}^{\floor{p}}\Big),\label{eq:roughpathincrements}\\
% %X_{s,t}^k & := \pi_k\big(X_{s,t}\big),\nonumber
% %\end{align}
% %where $\pi_k : T^{\floor{p}}\big(\R^d\big)\rightarrow \big(\R^d\big)^{\otimes k}$ is the projection map onto $\big(\R^d\big)^{\otimes k}$, such that there exists a sequence of
% %continuous finite variation paths $x_n : [0,T] \rightarrow \R^d$ whose truncated signatures converge to $X$ in the $p$-variation metric:
% %\begin{equation}
% %d_p\Big(S_{0,T}^{\floor{p}}(x_n), X\Big) \rightarrow 0,
% %\label{eq:rpconvege}
% %\end{equation}
% %as $n\rightarrow\infty$, where the $p$-variation between two continuous paths $Z^1$ and $Z^2$ in $T^{\floor{p}}(\R^d)$ is
% %\begin{equation}
% %d_p\big(Z_1, Z_2\big) := \max_{1\leq k\leq \floor{p}}\sup_{\D}\bigg(\sum_{t_i\in\D}\Big\|\pi_k\big(Z_{t_i, t_{i+1}}^1\big) - \pi_k\big(Z_{t_i, t_{i+1}}^2\big)\Big\|^p\bigg)^\frac{1}{p},
% %\label{eq:rpmetric}
% %\end{equation}
% %where the supremum is taken over all partitions $\D$ of $[0,T]$ and the norms $\|\cdot\|$ must satisfy (up to some constant)
% %\begin{equation}
% %\|a\otimes b\| \leq \|a\|\|b\|,\nonumber
% %\end{equation}
% %for $a\in(\R^d)^{\otimes n}$ and $b\in(\R^d)^{\otimes m}$. For example, we can take $\|\cdot\|$ to be the projective or injective tensor norms (Prop 2.1 and Prop 3.1 in \cite{tensorproducts2002book}).
% %
% %\item The solution $Y$ and its initial value $\xi$ both take their values in $\R^n$.
% %
% %\item The collection of vector fields $\{f_1, \cdots, f_d\}$ on $\R^n$ are denoted by $f : \R^n\rightarrow L(\R^n, \R^d)$,
% %where $L(\R^n, \R^d)$ is the space of linear maps from $\R^n$ to $\R^d$. We will assume that $f$ has $Lip(\gamma)$ regularity with $\gamma > p$.
% %That is, the following norm is finite:
% %\begin{equation}
% %\|f\|_{Lip(\gamma)} := \max_{0 \leq k\leq \floor{\gamma}}\big\|D^k f\big\|_{\infty} \vee \big\|D^{\floor{\gamma}} f\big\|_{(\gamma - \floor{\gamma})-\text{H\"{o}l}}\,,
% %\label{eq:lipgamma}
% %\end{equation}
% %where $D^k f$ is the $k$-th (Fr\'{e}chet) derivative of $f$ and $\|\cdot\|_{\alpha\text{-H\"{o}l}}$ is the standard $\alpha$-H\"{o}lder norm for $\alpha\in(0,1)$.
% %
% %\item The rough differential equation \ref{eq:RDE} is defined in the Lyon's sense \cite{roughpath1998def}, so by the Universal Limit Theorem
% %(Theorem 5.3 in \cite{roughpath2007notes}), there exists a unique solution $Y : [0,T]\rightarrow\R^n$.
% %\end{itemize}
% %
% %We then define a specific ODE for approximating the solution $Y$ over an interval $[s,t]\subset [0,T]$.
% %\begin{enumerate}
% %\item Compute the $\floor{\gamma}$-step log-signature of the driving path $X$ over $[s,t]$. That is, we obtain $\log_{\floor{\gamma}}\big(S_{s,t}^{\floor{\gamma}}(X)\big) \in T^{\floor{\gamma}}(\R^d)$, where $\log_{\floor{\gamma}}(\cdot)$ is defined by projecting the standard tensor logarithm map onto $\{a\in T^{\floor{\gamma}}(\R^d) : \pi_0(a)>0\}$.
% %
% %\item Define the vector field derivatives $f^{\circ k} : \R^n\rightarrow L((\R^d)^{\otimes k}$ recursively by
% %\begin{align}
% %f^{\circ (1)}(y) & := f(y),\label{eq:derivatives}\\
% %f^{\circ (k + 1)}(y) & := D\big(f^{\circ k}\big)(y)f(y),\nonumber
% %\end{align}
% %for $y\in\R^n$.
% %
% %\item Construct the following (well-posed) ODE on the interval $[0,1]$,
% %\begin{align}
% %\frac{dz^{s,t}}{du} & := F\big(z^{s,t}\big),\label{eq:standardlogode}\\
% %z_0^{s,t} & := Y_s,\nonumber
% %\end{align}
% %where the vector field $F:\R^n\rightarrow\R^n$ is defined from the log-signature as
% %\begin{equation}
% %F(z) := \sum_{k=1}^{\floor{\gamma}}f^{\circ k}(z)\pi_k\Big(\log_{\floor{\gamma}}\big(S_{s,t}^{\floor{\gamma}}(X)\big)\Big).
% %\label{eq:logodevectfield}
% %\end{equation}
% %\end{enumerate}
% %Then we can approximate $Y_t$ using the $u = 1$ solution of (\ref{eq:standardlogode}). Moreover, there exists a universal constant $C_{p,\gamma}$ depending only on $p$ and $\gamma$ such that 
% %\begin{equation}
% %\big\|Y_t - z_1^{s,t}\big\| \leq C_{p,\gamma}\|f\|_{Lip(\gamma)}^\gamma\|X\|_{p\text{-var};[s,t]}^\gamma,
% %\label{eq:local_logodeestimate}
% %\end{equation}
% %where $\|\cdot\|_{p\text{-var};[s,t]}$ is the $p$-variation norm defined for paths in $T^{\floor{p}}(\R^d)$ by
% %\begin{equation}
% %\|X\|_{p\text{-var};[s,t]} := \max_{1\leq k\leq \floor{p}}\sup_{\D}\bigg(\sum_{t_i\in\D}\big\|X_{t_i, t_{i+1}}^k\big\|^p\bigg)^\frac{1}{p},
% %\label{eq:rpnorm}
% %\end{equation}
% %with the supremum taken over all partitions $\D$ of $[s,t]$.
% %\end{theorem}\medbreak
% %\begin{remark}
% %If the vector fields $\{f_1, \cdots, f_d\}$ are linear, then it is a straightforward exercise to show that $F$ is linear.
% %\end{remark}
% %
% %Although the above theorem requires some sophisticated theory, it has a simple conclusion - namely
% %that log-ODEs can approximate controlled differential equation. That said, the estimate (\ref{eq:local_logodeestimate}) does not directly apply when the vector fields $\{f_i\}$ are linear as they are unbounded. Fortunately, it is well-known that solutions of linear RDEs exist and are unique.
% %\begin{theorem}[Theorem 10.57 in \cite{friz2010multidimensional}]\label{thm:linearexistance}
% %Consider the linear RDE on $[0,T]$
% %\begin{align}
% %dY_t & = f(Y_t)\,dX_t,\label{eq:linearRDE2}\\
% %Y_0 & = \xi,\nonumber
% %\end{align}
% %where $X$ is a geometric $p$-rough path in $\R^d$, $\xi\in\R^n$ and the vector fields $\{f_i\}_{1\leq i\leq d}$ take the form $f_i(y) = A_i y + B$ where $\{A_{i}\}$ and $\{B_i\}$ are $n\times n$ matrices. Let $K$ denote an upper bound on $\max_i (\|A_i\| + \|B_i\|)$. Then a unique solution $Y:[0,T]\rightarrow\R^n$ exists. Moreover, it is bounded and there exists a constant $C_p$ depending only on $p$ such that
% %\begin{equation}
% %\|Y_t - Y_s\| \leq C_p\big(1+\|\xi\|\big)K\|X\|_{p\text{-var};[s,t]}\exp\Big(C_p K^p \|X\|_{p\text{-var};[s,t]}^p\Big),
% %\label{eq:linearRDEbound}
% %\end{equation}
% %for all $0\leq s\leq t\leq T$.
% %\end{theorem}
% %
% %When the vector fields of the RDE (\ref{eq:RDE}) are linear, then the log-ODE (\ref{eq:standardlogode}) also becomes linear. Therefore, the log-ODE solution exists and is explicitly given as the exponential of the matrix $F$.
% %
% %\begin{theorem}
% %Consider the same linear RDE on $[0,T]$ as in Theorem \ref{thm:linearexistance},
% %\begin{align}
% %dY_t & = f(Y_t)\,dX_t,\label{eq:linearRDE1}\\
% %Y_0 & = \xi.\nonumber
% %\end{align}
% %Then the log-ODE vector field $F$ given by (\ref{eq:logodevectfield}) is linear and the solution of the associated ODE (\ref{eq:standardlogode}) exists and satisfies
% %\begin{equation}
% %\|z_u^{s,t}\| \leq \|Y_s\|\exp\bigg(\sum_{m=1}^{\floor{\gamma}}K^m \Big\|\pi_m\Big(\log_{\floor{\gamma}}\big(S_{s,t}^{\floor{\gamma}}(X)\big)\Big)\Big\|\bigg),
% %\label{eq:linearODEbound}
% %\end{equation}
% %for $u\in[0,1]$ and all $0\leq s\leq t\leq T$.
% %\end{theorem}
% %\begin{proof}
% %Since $F$ is a linear vector field on $\R^n$, we can view it as an $e\times e$ matrix and so for $u\in[0,1]$,
% %\begin{equation}
% %z_u^{s,t} = \exp(uF)z_0^{s,t},\nonumber
% %\end{equation}
% %where $\exp$ denotes the matrix exponential. The result now follows by the standard estimate $\|\exp(F)\| \leq \exp(\|F\|)$.
% %\end{proof}
% %\begin{remark}\label{rmk:linear_rmk}
% %By the boundedness of linear RDEs (\ref{eq:linearRDEbound}) and log-ODEs (\ref{eq:linearODEbound}), the arguments that established Theorem \ref{thm:logODEthm} will hold in the linear case as $\|f\|_{Lip(\gamma)}$ would be finite when defined using the domains that the solutions $Y$ and $z$ lie in.
% %\end{remark}
% %
% %Given the local error estimate (\ref{eq:local_logodeestimate}) for the log-ODE method, we can now consider the approximation error that is exhibited by a log-ODE numerical solution to the RDE (\ref{eq:RDE}). Fortunately, the analysis required to derive such global error estimates was developed by Greg Gyurk\'{o} in his PhD thesis \cite{gyurko2008thesis}. 
% %Thus, the following result is a straightforward application of Theorem 3.2.1 from \cite{gyurko2008thesis}.\medbreak
% %
% %\begin{theorem} Let $X$, $f$ and $Y$ satisfy the assumptions given by Theorem \ref{thm:logODEthm} and suppose that $\{0 = t_0 < t_1 < \cdots < t_N = T\}$ is a partition of $[0,T]$ with $\max_{\,k}\|X\|_{p\text{-var};[t_k,t_{k+1}]}$ sufficiently small. We can construct a numerical solution $\{Y_k^{Log}\}_{0\leq k \leq N}$ of (\ref{eq:RDE}) by setting $Y_0^{Log} := Y_0$ and for each $k \in \{0, 1, \cdots, N - 1\}$, defining $Y_{k+1}^{Log}$ to be the solution at $u=1$ of the following ODE:
% %\begin{align}
% %\frac{dz^{t_k,t_{k+1}}}{du} & := F\big(z^{t_k,t_{k+1}}\big),\label{eq:standardlogode2}\\
% %z_0^{t_k,t_{k+1}} & := Y_k^{Log},\nonumber
% %\end{align}
% %where the vector field $F$ is constructed from the log-signature of $X$ over the interval $[t_k, t_{k+1}]$ according to (\ref{eq:logodevectfield}). Then there exists a constant $C$ depending only on $p$, $\gamma$ and $\|f\|_{Lip(\gamma)}$ such that
% %\begin{equation}
% %\big\|Y_{t_k} - Y_k^{Log}\big\| \leq C\sum_{i=0}^{k-1}\|X\|_{p\text{-var};[t_i,t_{i+1}]}^\gamma,
% %\label{eq:global_logodeestimate}
% %\end{equation}
% %for $0\leq k\leq N$.
% %\end{theorem}
% %\begin{remark}
% %The above error estimate also holds when the vector field $f$ is linear (by remark \ref{rmk:linear_rmk})).
% %\end{remark}
% %
% %[Talk about computational complexity, i.e. using more log-signature gives high order convergence...]
